# Supplementary material for: Earth Mover's Distance as a metric to evaluate the extent of charge transfer in excitations using discretized real-space densities
Source: arXiv:2308.07544 ancillary file (2023-10-07)
Supplement: Supplementary file 1 [file SI.pdf]

# Supporting Information: Earth Mover's Distance as a metric to evaluate the extent of charge transfer in excitations based on discrete real space density

Zhe Wang,[†,¶] Jiashu Liang,[†,¶] and Martin Head-Gordon[*,†,‡]

† *Kenneth S. Pitzer Center for Theoretical Chemistry, Department of Chemistry, University of California at Berkeley, Berkeley, CA 94720, USA*

‡ *Chemical Sciences Division, Lawrence Berkeley National Laboratory, Berkeley, CA 94720, USA*

¶ *These authors contributed equally to this work.*

E-mail: mhg@cchem.berkeley.edu

# 1 Accuracy of the quadrature grid - (50,194) vs SG-3

**Table S1:** Error in $\mu^{\mathrm{EMD}}$ and the excitation energy between TDDFT calculations under quadrature grids (50,194) and SG-3. CAM-B3LYP is used as the functional in the calculations.

| Molecule | Multiplicity | Excitation type | Strength | Symmetry | Symmetry of occupied orbitals | Error in $\mu^{\mathrm{EMD}}$ | Error in Excitation energy (eV) |
|---|---|---|---|---|---|---|---|
| Aminobenzonitrile | Singlet | CT | 0.447 | $A_1$ | $B_2$ | 0.003 | -0.001 |
| Aniline | Singlet | CT | 0.175 | $A_1$ | $A_2$ $B_2$ | 0.006 | -0.002 |
| Azulene | Singlet | CT | 0.003 | $A_1$ | $B_2$ $A_2$ | 0.0 | 0.0 |
| Azulene | Singlet | CT | 0.055 | $B_1$ | $A_2$ $B_2$ | 0.0 | 0.0 |
| Benzene | Triplet | V | | $B_{1u}$ | | 0.001 | 0.0 |
| Benzene | Singlet | V | | $B_{2u}$ | | 0.0 | -0.0 |
| Benzene | Singlet | R | | $E_{1g}$ | | 0.018 | -0.009 |
| Benzene | Singlet | R | 0.066 | $A_2$u | | 0.011 | -0.006 |
| Benzonitrile | Singlet | CT | | $A_2$ | $B_1$ | 0.0 | -0.0 |
| Benzothiadiazole | Singlet | CT | 0.058 | $B_1$ | $A_2$ | 0.001 | -0.0 |
| Carbon monoxide | Triplet | V | | $\Pi$ | $\Sigma$ | -0.0 | -0.001 |
| Carbon monoxide | Singlet | V | 0.084 | $\Pi$ | $\Sigma$ | 0.017 | -0.002 |
| Carbon monoxide | Singlet | R | 0.003 | $\Sigma^+$ | $\Sigma$ | -0.01 | -0.009 |
| Carbon monoxide | Triplet | R | | $\Sigma^+$ | $\Sigma^+$ | -0.002 | -0.01 |
| Cyclopropene | Triplet | V | | $B_1$ | $B_2$ | -0.001 | 0.0 |
| Cyclopropene | Singlet | V | 0.001 | $B_2$ | $B_1$ | 0.024 | -0.001 |
| Dimethylaminobenzonitrile | Singlet | CT | 0.585 | $A_1$ | $B_2$ | 0.001 | -0.0 |
| Dimethylaniline | Singlet | CT | 0.042 | $B_1$ | $B_2$ | -0.0 | 0.0 |
| Dimethylaniline | Singlet | CT | 0.319 | $A_1$ | $B_2$ | -0.02 | -0.008 |
| Ethylene | Triplet | V | | $B_{3u}$ | $B_{1u}$ | 0.0 | 0.0 |
| Ethylene | Singlet | R | 0.078 | $B_{1u}$ | $B_{1u}$ | 0.006 | -0.005 |
| Ethylene | Singlet | R | | B3g | $B_{1u}$ | -0.004 | -0.004 |
| Ethylene | Triplet | R | | $B_{1u}$ | $B_{1u}$ | 0.005 | -0.004 |
| Furan | Triplet | V | | $B_1$ | $A_2$ $B_2$ | 0.002 | 0.0 |
| Furan | Singlet | R | | $A_2$ | $A_2$ | 0.008 | -0.009 |
| HCl | Singlet | CT | 0.056 | $\Pi$ | | 0.002 | -0.002 |
| HCOOH | Singlet | core | 0.01 | $A'$ | $A'$ | 0.002 | -0.067 |
| Imidazole | Singlet | core | 0.009 | $A'$ | $A'$ | 0.002 | -0.036 |
| Naphthalene | Singlet | V | 0.0 | $B_{3u}$ | Au | 0.0 | 0.0 |
| Naphthalene | Singlet | V | 0.067 | $B_{2u}$ | Au | 0.0 | 0.0 |
| Naphthalene | Singlet | R | | Au | Au | 0.012 | -0.012 |
| Naphthalene | Singlet | R | | $B_2$g | Au | 0.018 | -0.006 |
| Naphthalene | Singlet | V | | $B_1$g | Au | 0.008 | -0.002 |
| Naphthalene | Singlet | R | | B3g | Au | 0.01 | -0.008 |
| Nitroaniline | Singlet | CT | 0.41 | $A_1$ | $B_2$ | -0.003 | -0.0 |
| Nitrobenzene | Singlet | CT | 0.214 | $A_1$ | $B_2$ | 0.0 | 0.0 |
| Nitrodimethylaniline | Singlet | CT | 0.511 | $A_1$ | $B_2$ | 0.0 | -0.0 |
| Nitropyridine N-Oxide | Singlet | CT | 0.422 | $A_1$ | $B_2$ | 0.0 | 0.0 |
| N-Phenylpyrrole | Singlet | CT | 0.017 | $B_1$ | $A_2$ | -0.002 | -0.001 |
| N-Phenylpyrrole | Singlet | CT | 0.237 | $A_1$ | $A_2$ | 0.0 | 0.0 |
| $PF_3$ | Singlet | core | 0.006 | $A''$ | $A'$ | 0.0 | -1.074 |
| Phthalazine | Singlet | CT | | $A_2$ | $B_1$ | -0.0 | -0.0 |
| Phthalazine | Singlet | CT | 0.005 | $B_2$ | $B_1$ | -0.0 | 0.0 |
| Pyridine | Triplet | V | | $A_1$ | $A_2$ | -0.0 | 0.0 |
| Pyridine | Singlet | V | 0.004 | $B_2$ | $A_1$ | 0.0 | -0.0 |
| Pyridine | Singlet | R | | $A_2$ | $A_2$ | 0.0 | -0.01 |
| Pyridine | Singlet | R | 0.011 | $A_1$ | $A_1$ | -0.01 | -0.013 |
| Pyridine | Singlet | R | 0.045 | $B_2$ | $A_2$ | -0.002 | -0.006 |
| Quinoxaline | Singlet | CT | 0.034 | $B_1$ | $A_2$ | -0.0 | -0.0 |
| Quinoxaline | Singlet | CT | 0.374 | $A_1$ | $B_2$ $A_2$ | 0.001 | -0.0 |
| Quinoxaline | Singlet | CT | 0.003 | $B_2$ | $A_1$ | -0.0 | -0.0 |
| $SiMe_4$ | Singlet | core | | $A_1$ | $A_1$ | -0.034 | -0.783 |
| Streptocyanine-C1 | Triplet | V | | $B_1$ | $A_2$ | -0.0 | 0.0 |
| Streptocyanine-C1 | Singlet | V | 0.347 | $B_1$ | $A_2$ | -0.0 | 0.0 |
| Streptocyanine-C3 | Triplet | V | | $B_1$ | $B_2$ | -0.0 | 0.0 |
| Streptocyanine-C3 | Singlet | V | 0.755 | $B_1$ | $B_2$ | -0.0 | 0.0 |
| Streptocyanine-C5 | Triplet | V | | $B_1$ | $A_2$ | -0.0 | 0.0 |
| Streptocyanine-C5 | Singlet | V | 1.182 | $B_1$ | $A_2$ | -0.001 | 0.0 |
| Twisted Dimethylaniline | Singlet | CT | | $A_2$ | $B_1$ | -0.0 | -0.001 |
| Twisted Dimethylaniline | Singlet | CT | 0.0 | $B_2$ | $B_1$ | 0.003 | -0.001 |
| Twisted N-Phenylpyrrole | Singlet | CT | 0.001 | $B_1$ | $A_2$ $B_2$ $A_2$ | 0.002 | -0.001 |
| Twisted N-Phenylpyrrole | Singlet | CT | 0.008 | $A_1$ | $A_2$ | 0.0 | -0.0 |
| Twisted N-Phenylpyrrole | Singlet | CT | | $A_2$ | $B_1$ | -0.001 | -0.0 |
| Twisted N-Phenylpyrrole | Singlet | CT | 0.008 | $B_2$ | $B_1$ | -0.006 | -0.001 |
| Water | Triplet | R | | $B_2$ | $B_2$ | 0.001 | -0.001 |
| Water | Singlet | R | 0.054 | $B_2$ | $B_2$ | 0.001 | -0.001 |
| Water | Singlet | core | 0.008 | $A_1$ | $A_1$ | 0.002 | -0.059 |
| | | | | | RMSE | 0.008 | 0.163 |

## 2 Charge-transfer excitations with the nature of Rydberg excitation in the data set

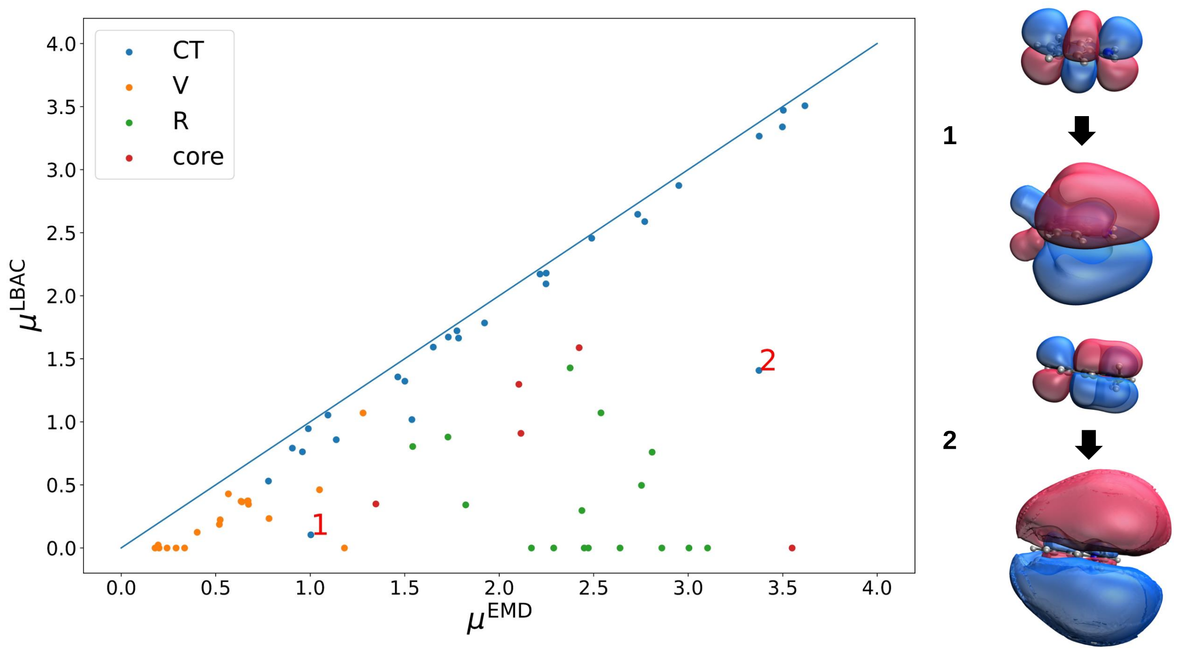


**Figure S1:** Natural transition orbitals (NTOs) of the charge-transfer (CT) excitation states with a large $\mu^{\mathrm{EMD}}$-$\mu^{\mathrm{LBAC}}$ ratio. For each NTO pair, the top one is the highest occupied (HO) NTO and the bottom one is the lowest unoccupied (LU) NTO. The isovalue of the surface is set to be 0.01 Å$^{-3}$. The blue line represents a slope of 1, indicating a one-to-one relationship. Data points **1** and **2** correspond to aniline and dimethylaniline respectively, whose NTOs are shown on the right of the figure.

From the NTOs for aniline (**1**) and dimethylaniline (**2**) shown in Figure S1, some CT excitation states in our data set are demonstrated to have partial Rydberg character, resulting in a large $\mu^{\mathrm{EMD}}$ to $\mu^{\mathrm{LBAC}}$ ratio. This is also evidence that the extent of (pseudo-)centrosymmetry of an excitation can be distinguished by examining the $\mu^{\mathrm{EMD}}$:$\mu^{\mathrm{LBAC}}$ ratio. As discussed in the main text, $\mu^{\mathrm{LBAC}}$ vanishes for centro-symmetric excitations, while $\mu^{\mathrm{EMD}}$ does not.

# 3 Comparison of $\mu^{\text{LBAC}}$ and $\mu^{\text{RMS}}$ from different theories

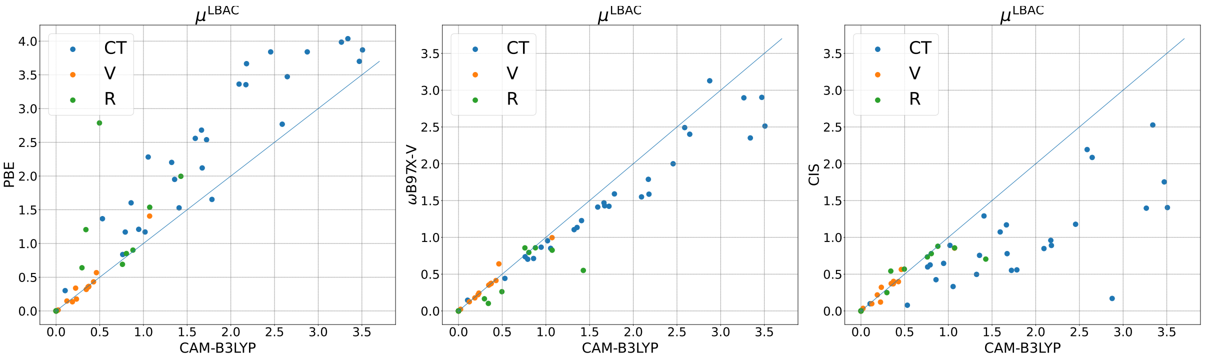


**Figure S2:** Comparison of $\mu^{\text{LBAC}}$ values evaluated from densities calculated from different theoretical methods incorporating various Hartree-Fock (HF) exchange components (PBE, CAM-B3LYP, $\omega$B97X-V, and CIS). The blue line represents a slope of 1, indicating a one-to-one relationship.

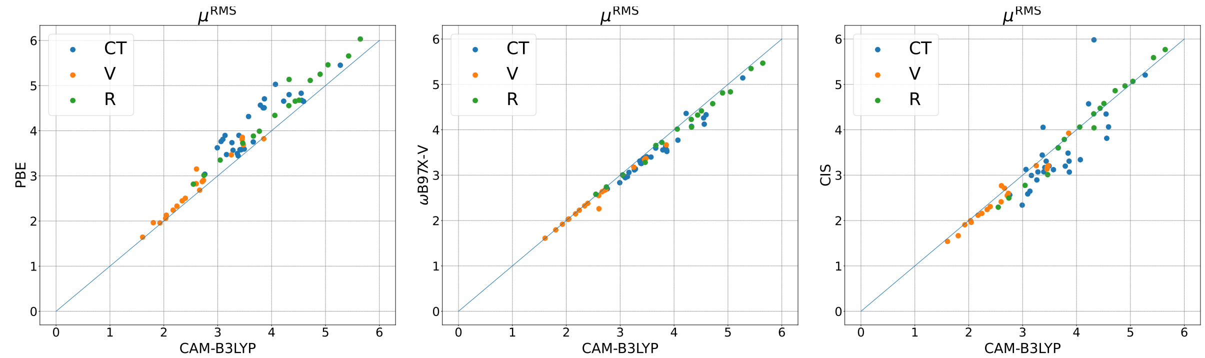


**Figure S3:** Comparison of $\mu^{\text{RMS}}$ values evaluated from densities calculated from different theoretical methods incorporating various HF exchange components (PBE, CAM-B3LYP, $\omega$B97X-V, and CIS). The blue line represents a slope of 1, indicating a one-to-one relationship.

Figure S2 compares the $\mu^{\text{LBAC}}$ values evaluated from the electronic densities generated by TDDFT calculations using PBE, CAM-B3LYP, and $\omega$B97X-V as the functional, as well as CIS. A parallel comparison for $\mu^{\text{RMS}}$ is also depicted in Figure S3. For most CT states, theories with substantial HF exchange components are associated with lower metric values, signifying that predictions of charge-hole separation extent tend to decrease with increasing

fractions of exact (HF) exchange. Inspection of these figures reveals that $\mu^{\mathrm{RMS}}$ displays less sensitivity to theory alteration, due to the relatively consistent sizes of the electron and hole for the same excitation across different theories.

# 4 Application of $\mu^{\text{EMD}}$ in assigning correct excited states in TDDFT calculations

The inherent inaccuracy of quantum chemistry methods means that identical excited states (in terms of excitation energy, excited state density and wavefunction, etc) are seldom produced by different theories. At times, the discrepancy between these states, neither overly large nor extremely small, creates a challenge in determining whether the two states are identical or not between two methods. While NTOs can effectively elucidate these differences and similarities, manually examining them becomes unwieldy with a large number of excitations. As a metric for the distribution differences, $\mu^{\text{EMD}}$ could work as an auxiliary tool in assigning excited states and distinguishing differences alongside the symmetry, excitation strength, and excitation energy.

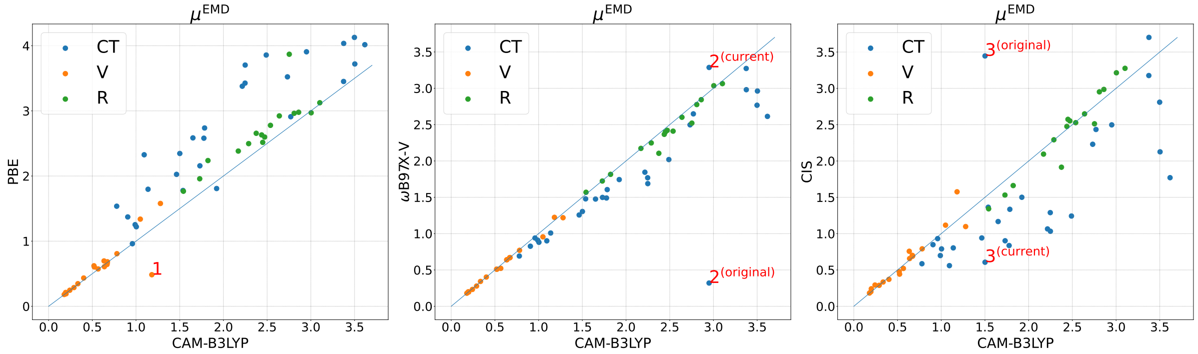


**Figure S4:** Figure 6 showing with some incorrectly assigned states previously. Comparison of $\mu^{\text{EMD}}$s based on density calculated from theoretical methods with different Hartree-Fock (HF) exchange components (PBE, CAM-B3LYP, $\omega$B97X-V, and CIS). The blue line represents a slope of 1, indicating a one-to-one relationship.

When examining the influence of different functionals on $\mu^{\text{EMD}}$ in TDDFT calculations, we detected some outliers, which are labeled in Figure S4. Point 1 represents a valence excitation in naphthalene. For this excitation, the HONTO calculated by PBE looks similar to the one calculated by CAM-B3LYP (See Figure S5). Their LUNTOs differ somewhat

nonetheless, since the naphthalene LUNTO under CAM-B3LYP displays an enrichment of charge density between the $\alpha$-Hs. As we failed to identify a state with a more similar LUNTO, we surmise that these two excitations are the same. From Table S2, we observe that $\mu^{\mathrm{LBAC}}$ is zero since it is a centrosymmetric excitation. $\mu^{\mathrm{RMS}}$ gives similar results as both the hole size and electron size exhibit little variation. In contrast, $\mu^{\mathrm{EMD}}$ captures the difference between the two excitations (i.e. 1 and 2 in Figure S5), as it is much smaller for the excited state calculated using PBE, wherein less charge is transported to the middle of the $\alpha$-Hs.

**Table S2:** Theoretical metrics and TDDFT excitation energy of of the excited states highlighted in Figure S4

| Point in Figure S4 | Molecule | Excitation type | Theory | Index in Figure S5 | Description | $\mu^{\mathrm{EMD}}$ | $\mu^{\mathrm{LBAC}}$ | $\mu^{\mathrm{RMS}}$ | Excitation energy (eV) |
|---|---|---|---|---|---|---|---|---|---|
| 1 | Naphthalene | V | CAM-B3LYP | 1 | Reference state | 1.181 | 0 | 3.855 | 5.989 |
| | | | PBE | 2 | Currently assigned state | 0.485 | 0 | 3.823 | 4.995 |
| 2 | Twisted N-Phenylpyrrole | CT | CAM-B3LYP | 3 | Reference state | 2.950 | 2.875 | 4.224 | 5.342 |
| | | | $\omega$B97X-V | 4 | Previously assigned state[S1] | 0.320 | 0.163 | 2.768 | 5.591 |
| | | | $\omega$B97X-V | 5 | Currently assigned state | 3.287 | 3.128 | 4.360 | 6.052 |
| 3 | Benzonitrile | CT | CAM-B3LYP | 6 | Reference state | 1.501 | 1.323 | 2.992 | 6.615 |
| | | | CIS | 7 | Previously assigned state[S1] | 3.446 | 0.833 | 5.332 | 7.748 |
| | | | CIS | 8 | Currently assigned state | 0.607 | 0.497 | 2.340 | 6.869 |

We discovered the other two outliers (Point 2 and Point 3 in Figure S4) are mismatched excited states that were incorrectly assigned in Ref. S1. We now correct them using based on $\mu^{\mathrm{EMD}}$ values and inspection of the NTOs. The reassigned states display more reasonable $\mu^{\mathrm{EMD}}$, $\mu^{\mathrm{LBAC}}$, and $\mu^{\mathrm{RMS}}$ values. The reassignment is also supported by comparing each corresponding NTO pair (3-5 and 6-8 in Figure S5). For the CT excitation in benzonitrile, the newly matched state shows small $\mu^{\mathrm{EMD}}$ and $\mu^{\mathrm{LBAC}}$ values, which aligns with the discussion in Section 3.3: theories with higher HF exchange proportions generally predict a smaller degree of charge-hole separation for long-range CT excitations. $\mu^{\mathrm{RMS}}$ follows the same trend as $\mu^{\mathrm{LBAC}}$ and $\mu^{\mathrm{EMD}}$, although with less sensitivity.

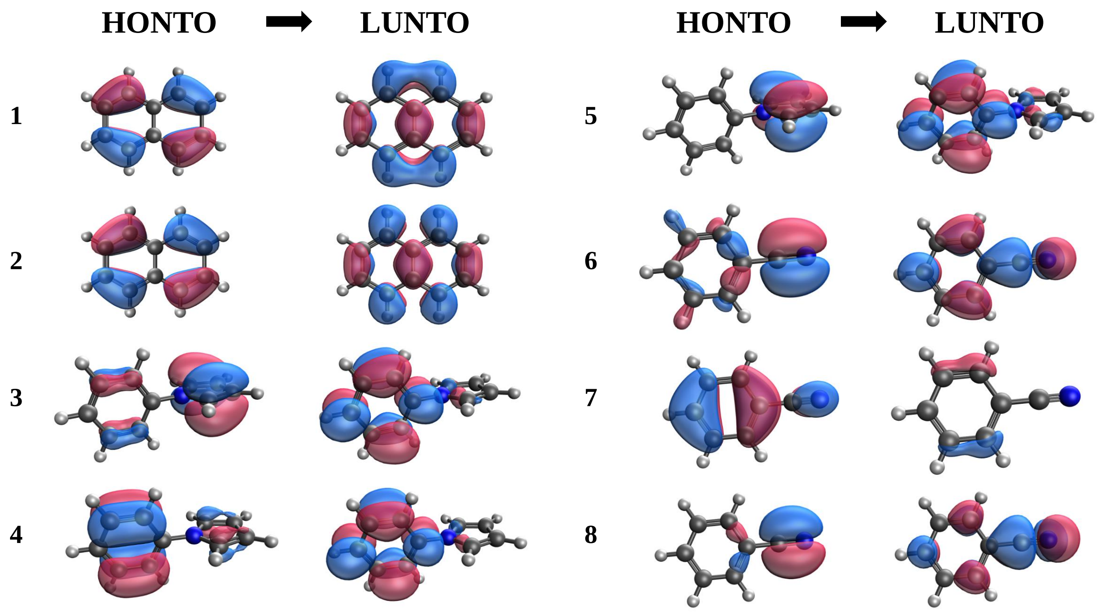


**Figure S5:** NTOs corresponding to the excitations indexed in Table S2. The isovalue of the surface is set to be 0.1 Å$^{-3}$.

# 5 Comparison among $q^{\mathrm{CT}}$, $d^{\mathrm{EMD}}$, and $\mu^{\mathrm{EMD}}$ as the metric for functional performance assessment

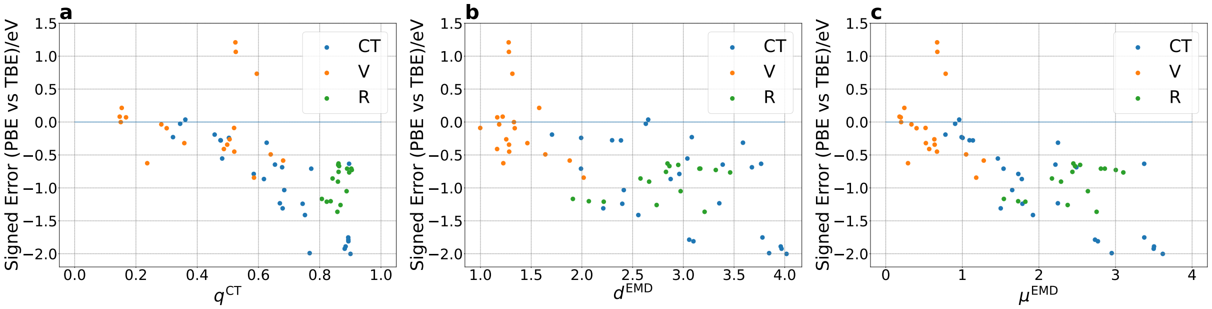


**Figure S6:** The relationship between the PBE's signed error and the three metrics ($q^{\mathrm{CT}}$, $d^{\mathrm{EMD}}$, and $\mu^{\mathrm{EMD}}$) in TDDFT calculations. The metrics are computed from densities generated using the CAM-B3LYP functional.

A comparison among $q^{\mathrm{CT}}$, $d^{\mathrm{EMD}}$, and $\mu^{\mathrm{EMD}}$ is given in Figure S6. A notable observation is the evident relationship between the PBE's signed error and $q^{\mathrm{CT}}$. However, there's a significant overlap between valence-excited states and short-range CT excited states, complicating the identification of the commencement point of semi-local functionals' failures. This scenario also resonates with the $\Lambda$[S2] and $\phi_S$[S3] metrics (see Figure 2 in Ref. S2), given the roughly quadratic relationship between $q^{\mathrm{CT}}$ and $\phi_S$.[S4] As a topological metric, $d^{\mathrm{EMD}}$ establishes a relatively clear differentiation between the two kinds of excitations, i.e., the valence excitations and the short-range CT excitations. Further scrutiny reveals that PBE tends to underestimate when $d^{\mathrm{EMD}}$ exceeds 1.5. Nonetheless, post this threshold, the magnitude seems unrelated to PBE's signed error. Given these observations, it becomes logical to introduce $\mu^{\mathrm{EMD}}$—a product of $q^{\mathrm{CT}}$ and $d^{\mathrm{EMD}}$—as a refined metric to evaluate functional performance. This new metric can capture the nuanced relationship between CT error and the transferred charge, while maintaining a precise distinction between valence and short-range CT excitations.

# 6 Performance of functionals in TDDFT calculations taking $\mu^{\mathrm{EMD}}$ as the metric for density difference evaluation

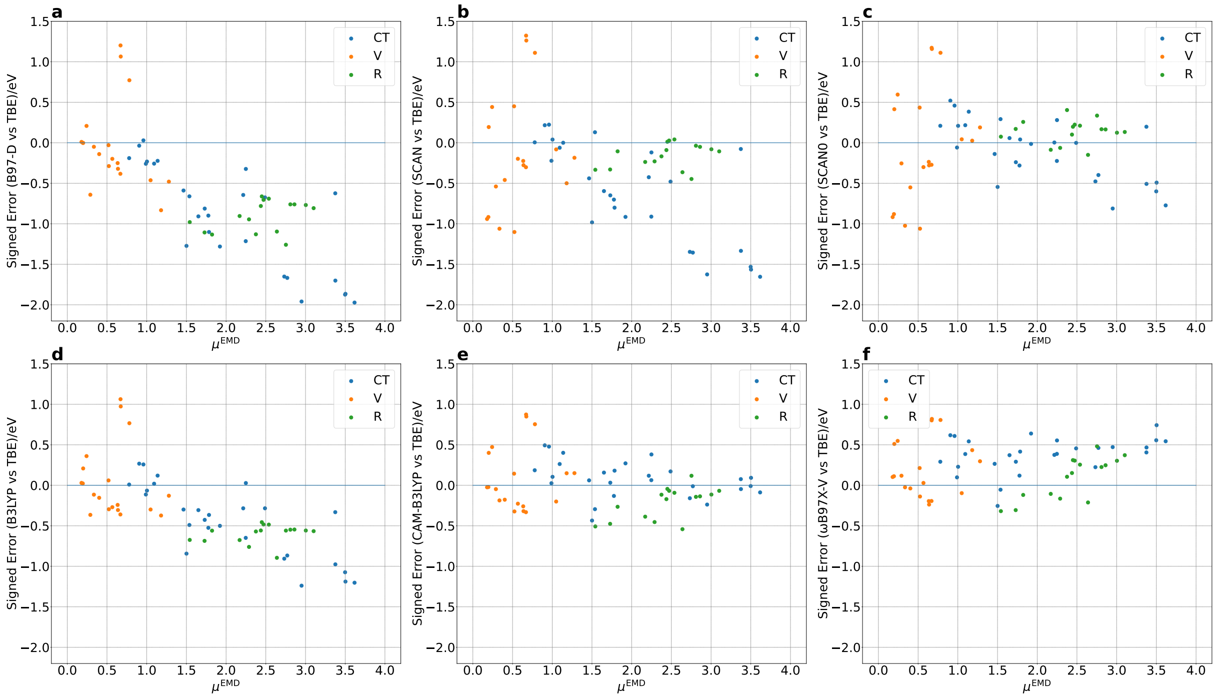


**Figure S7:** Comparisons of the performance of more functionals in TDDFT excitation energies. $\mu^{\mathrm{EMD}}$ is computed from densities generated in the TDDFT calculation using the CAM-B3LYP functional. The presented functionals include B97-D,[S5] SCAN,[S6] SCAN0,[S7] B3LYP,[S8] CAM-B3LYP,[S9] and $\omega$B97X-V.[S10]

# 7 Relationship of $||\mu^{\mathbf{LBAC}}||$, $|\mathbf{r}_e - \mathbf{r}_h|$, and $\Delta r$ (for CIS and TDDFT/TDA)

In this section, we report some formal results connecting different CT metrics for the special case where the excitation is represented through the Tamm-Dancoff approximation to TDDFT or CIS, which is the corresponding wavefunction theory. For simplicity, we take all AOs and MOs to be real. We also work in the spin-orbital basis.

## 7.1 Notation

Index conventions:

- $i, j, \cdots$ correspond to occupied molecular orbitals (MOs), $\phi_i$, $\phi_j$
- $a, b, \cdots$ correspond to virtual MOs, $\phi_a$, $\phi_b$
- $\mu, \nu, \lambda, \cdots$ correspond to atomic orbitals (AOs) $\omega_\mu, \omega_\nu, \omega_\lambda, \cdots$

Symbols:

- $\Phi^0$ is the HF ground state wavefunction
- $\Phi^I$ is the TDA/CIS wavefunction for the $I^{\text{th}}$ excited state
- $t_i^a$ is the TDA/CIS amplitude of the substituted Slater determinant, $\Phi_i^a$, for state $I$
- $\chi_{\text{exc}}$ is the exciton wavefunction
- $\mathbf{D}_{\mu\nu}^{0I}$ are matrix elements of the 1-TDM represented in the AO basis
- $\mathbf{C}$ is the MO coefficient matrix
- $\mathbf{S}$ is the AO overlap matrix.

### 7.2 $||\mu^{\mathbf{LBAC}}||$

We are going to represent $||\mu^{\text{LBAC}}||$ in terms of MOs and CIS coefficients.

First, we can get the ground state and electronic state electronic density ($\rho^{\text{GS}}$ and $\rho^{\text{EX}}$) utilizing the Slater-Condon rules.

$$\begin{aligned}\rho^{\text{GS}}(\mathbf{r}) &= \langle\Phi^0|\sum_i \delta(\mathbf{r}-\mathbf{r}_i)|\Phi^0\rangle \\ &= \sum_i \langle\phi_i|\delta(\mathbf{r}-\mathbf{r}_i)|\phi_i\rangle \\ &= \sum_i |\phi_i(\mathbf{r})|^2\end{aligned} \tag{1}$$

$$\begin{aligned}\rho^{\text{EX}}(\mathbf{r}) &= \langle\Phi^I|\sum_k \delta(\mathbf{r}-\mathbf{r}_k)|\Phi^I\rangle \\ &= \langle\sum_{ia} t_i^a\Phi_i^a|\sum_k \delta(\mathbf{r}-\mathbf{r}_k)|\sum_{jb} t_j^b\Phi_j^b\rangle \\ &= \sum_i |\phi_i(\mathbf{r})|^2 + \sum_{iab} t_i^a t_i^b \phi_a(\mathbf{r})\phi_b(\mathbf{r}) - \sum_{ija} t_i^a t_j^a \phi_j(\mathbf{r})\phi_i(\mathbf{r})\end{aligned} \tag{2}$$

The difference in the electronic density, $\Delta\rho$, associated with the excitation is

$$\begin{aligned}\Delta\rho(\mathbf{r}) &= \rho^{\text{EX}}(\mathbf{r}) - \rho^{\text{GS}}(\mathbf{r}) \\ &= \sum_{iab} t_i^a t_i^b \phi_a(\mathbf{r})\phi_b(\mathbf{r}) - \sum_{ija} t_i^a t_j^a \phi_j(\mathbf{r})\phi_i(\mathbf{r})\end{aligned} \tag{3}$$

We can now obtain $||\mu^{\text{LBAC}}||$ in terms of MOs and CIS coefficients:

$$\begin{aligned}||\mu^{\text{LBAC}}|| &= \left|\int \mathbf{r}\Delta\rho(\mathbf{r})d\mathbf{r}\right| \\ &= \left|\sum_{iab} t_i^a t_i^b \langle\phi_a|\mathbf{r}|\phi_b\rangle - \sum_{ija} t_i^a t_j^a \langle\phi_j|\mathbf{r}|\phi_i\rangle\right|\end{aligned} \tag{4}$$

### 7.3 $|\mathbf{r}_e - \mathbf{r}_h|$

The electron center $\mathbf{r}_e$ and hole center $\mathbf{r}_h$ are defined as

$$\begin{aligned}
\mathbf{r}_e &= \langle \chi_{\text{exc}} | \mathbf{r}_e | \chi_{\text{exc}} \rangle \\
&= \int\int \sum_{\mu\nu} \mathbf{D}^{0I}_{\mu\nu} \omega_\mu(\mathbf{r}_h)\omega_\nu(\mathbf{r}_e)\mathbf{r}_e \sum_{\sigma\lambda} \mathbf{D}^{0I}_{\sigma\lambda}\omega_\sigma(\mathbf{r}_h)\omega_\lambda(\mathbf{r}_e) d\mathbf{r}_h d\mathbf{r}_e \\
&= \sum_{\mu\nu\sigma\lambda} \mathbf{D}^{0I}_{\mu\nu}\mathbf{D}^{0I}_{\sigma\lambda} \int\int \omega_\mu(\mathbf{r}_h)\omega_\nu(\mathbf{r}_e)\mathbf{r}_e\omega_\sigma(\mathbf{r}_h)\omega_\lambda(\mathbf{r}_e) d\mathbf{r}_h d\mathbf{r}_e \\
&= \sum_{\mu\nu\sigma\lambda} \mathbf{D}^{0I}_{\mu\nu}\mathbf{D}^{0I}_{\sigma\lambda}\mathbf{S}_{\mu\sigma} \langle \omega_\nu | \mathbf{r} | \omega_\lambda \rangle
\end{aligned} \tag{5}$$

$$\begin{aligned}
\mathbf{r}_h &= \langle \chi_{\text{exc}} | \mathbf{r}_h | \chi_{\text{exc}} \rangle \\
&= \int \sum_{\mu\nu} \mathbf{D}^{0I}_{\mu\nu} \omega_\mu(\mathbf{r}_h)\omega_\nu(\mathbf{r}_e)\mathbf{r}_h \sum_{\sigma\lambda} \mathbf{D}^{0I}_{\sigma\lambda}\omega_\sigma(\mathbf{r}_h)\omega_\lambda(\mathbf{r}_e) d\mathbf{r}_h d\mathbf{r}_e \\
&= \sum_{\mu\nu\sigma\lambda} \mathbf{D}^{0I}_{\mu\nu}\mathbf{D}^{0I}_{\sigma\lambda} \int \omega_\mu(\mathbf{r}_h)\omega_\nu(\mathbf{r}_e)\mathbf{r}_h\omega_\sigma(\mathbf{r}_h)\omega_\lambda(\mathbf{r}_e) d\mathbf{r}_h d\mathbf{r}_e \\
&= \sum_{\mu\nu\sigma\lambda} \mathbf{D}^{0I}_{\mu\nu}\mathbf{D}^{0I}_{\sigma\lambda}\mathbf{S}_{\nu\lambda} \langle \omega_\mu | \mathbf{r} | \omega_\sigma \rangle
\end{aligned} \tag{6}$$

For CIS (and TDDFT/TDA), according to Slater-Condon rules, we have $\mathbf{D}^{0I}_{\mu\nu} = \sum_{ia} t^a_i \mathbf{C}_{\mu i}\mathbf{C}_{\nu a}$. Then we have

$$\begin{aligned}
\mathbf{r}_e &= \sum_{\mu\nu\sigma\lambda} \mathbf{D}^{0I}_{\mu\nu}\mathbf{D}^{0I}_{\sigma\lambda}\mathbf{S}_{\mu\sigma} \langle \omega_\nu | \mathbf{r} | \omega_\lambda \rangle \\
&= \sum_{\mu\nu\sigma\lambda} \sum_{ia} t^a_i \mathbf{C}_{\mu i}\mathbf{C}_{\nu a} \sum_{jb} t^b_j \mathbf{C}_{\sigma j}\mathbf{C}_{\lambda b}\mathbf{S}_{\mu\sigma} \langle \omega_\nu | \mathbf{r} | \omega_\lambda \rangle \\
&= \sum_{iajb} t^a_i t^b_j \sum_{\mu\sigma} \mathbf{C}_{\mu i}\mathbf{S}_{\mu\sigma}\mathbf{C}_{\sigma j} \sum_{\nu\lambda} \mathbf{C}_{\nu a} \langle \omega_\nu | \mathbf{r} | \omega_\lambda \rangle \mathbf{C}_{\lambda b} \\
&= \sum_{iajb} t^a_i t^b_j \langle \phi_i | \phi_j \rangle \langle \phi_a | \mathbf{r} | \phi_b \rangle \\
&= \sum_{iab} t^a_i t^b_i \langle \phi_a | \mathbf{r} | \phi_b \rangle
\end{aligned} \tag{7}$$

We can get $\mathbf{r}_h$ in the same way.

$$\mathbf{r}_h = \sum_{ija} t_i^a t_j^a \langle \phi_j | \mathbf{r} | \phi_i \rangle \tag{8}$$

So

$$|\mathbf{r}_e - \mathbf{r}_h| = \left| \sum_{iab} t_i^a t_i^b \langle \phi_a | \mathbf{r} | \phi_b \rangle - \sum_{ija} t_i^a t_j^a \langle \phi_j | \mathbf{r} | \phi_i \rangle \right| \tag{9}$$

We see that $|\mathbf{r}_e - \mathbf{r}_h|$ is exactly the same as $||\mu^{\text{LBAC}}||$.

If we are using the natural transition orbitals to represent the $\chi_{exc}$, then we can easily get another expression for $|\mathbf{r}_e - \mathbf{r}_h|$:

$$\begin{aligned} |\mathbf{r}_e - \mathbf{r}_h| = \Bigg| &\sum_{k_1 k_2} \sqrt{\lambda_{k_1}} \sqrt{\lambda_{k_2}} \sum_{iab} \mathbf{U}_{ik_1} \mathbf{U}_{ik_2} \mathbf{V}_{ak_1} \mathbf{V}_{bk_2} \langle \phi_a | \mathbf{r} | \phi_b \rangle \\ &- \sum_{k_1 k_2} \sqrt{\lambda_{k_1}} \sqrt{\lambda_{k_2}} \sum_{ija} \mathbf{U}_{ik_1} \mathbf{U}_{jk_2} \mathbf{V}_{ak_1} \mathbf{V}_{ak_2} \langle \phi_j | \mathbf{r} | \phi_i \rangle \Bigg| \end{aligned} \tag{10}$$

We have introduced the singular value decomposition of the 1-TDM as

$$\mathbf{D}^{0I} = \mathbf{U}\text{diag}(\sqrt{\lambda_1}, \sqrt{\lambda_2}, ...)\mathbf{V}^T. \tag{11}$$

## 7.4 $\Delta r$

Another metric for charge transfer is the distance $\Delta r$, introduced by Guido et al.[S11] and defined as:

$$\Delta r = \frac{\sum_{ia} t_i^{a2} |\langle \phi_a | \mathbf{r} | \phi_a \rangle - \langle \phi_i | \mathbf{r} | \phi_i \rangle|}{\sum_{ia} (t_i^a)^2} \tag{12}$$

If we can move the sum inside the absolute value, specifically if the difference $\langle \phi_a | \mathbf{r} | \phi_a \rangle - \langle \phi_i | \mathbf{r} | \phi_i \rangle$ is consistently non-negative or non-positive for all pairs of occupied-virtual orbitals that have a significant $t_i^a$ value, then this becomes the first term of $||\mu^{\text{LBAC}}||$ in the second line of (4). However, it lacks the second and third terms that account for the coupling between

different singly excited Slater determinants.

If NTOs are used instead of molecular orbitals, we have

$$
\begin{aligned}
\Delta r_{NTO} &= \frac{\sum_k^{Nocc} \lambda_k | \langle \phi_k^{I0} | \mathbf{r} | \phi_k^{I0} \rangle - \langle \phi_k^{0I} | \mathbf{r} | \phi_k^{0I} \rangle |}{\sum_k^{Nocc} \lambda_k} \\
&= \frac{\sum_k^{Nocc} \lambda_k | \langle \sum_a \mathbf{V}_{ak} \phi_a | \mathbf{r} | \sum_b \mathbf{V}_{bk} \phi_b \rangle - \langle \sum_i \mathbf{U}_{ik} \phi_i | \mathbf{r} | \sum_j \mathbf{U}_{jk} \phi_j \rangle |}{\sum_k^{Nocc} \lambda_k} \\
&= \frac{\sum_k^{Nocc} \lambda_k | \sum_{ab} \mathbf{V}_{ak} \mathbf{V}_{bk} \langle \phi_a | \mathbf{r} | \phi_b \rangle - \sum_{ij} \mathbf{U}_{ik} \mathbf{U}_{jk} \langle \phi_i | \mathbf{r} | \phi_j \rangle |}{\sum_k^{Nocc} \lambda_k}
\end{aligned}
\tag{13}
$$

In the above equation, $\phi_k^{I0}$ and $\phi_k^{0I}$ represent the electron and hole NTOs, respectively. If we can move the sum into the absolute value, $\Delta r_{NTO}$ is still not equal to $||\mu^{\text{LBAC}}||$ and $|\mathbf{r}_e - \mathbf{r}_h|$ since it lacks $\sum_{k1k2,k1\neq k2} \sqrt{\lambda_{k1}}\sqrt{\lambda_{k2}}$ terms.

# 8 Effect of Tamm-Dancoff approximation (TDA) on $\mu^{\text{EMD}}$

The existence of the de-excitation block in full TDDFT calculations may affect the distribution of the real space density and thus change the result of $\mu^{\text{EMD}}$. However, the extent of the de-excitation is usually small and does not affect the metric much. For instance, we randomly choose the four lowest CT excited states of twisted N-phenylpyrrole and show their $\mu^{\text{EMD}}$ metric values as below.

**Table S3:** TDDFT/TDA vs full TDDFT for twisted N-phenylpyrrole

| Excitation type | $\mu^{\text{EMD}}$ with TDA | $\mu^{\text{EMD}}$ without TDA | Relative difference in $\mu^{\text{EMD}}$% |
|---|---|---|---|
| CT | 3.90697 | 3.90490 | 0.053 |
| CT | 4.01633 | 3.99220 | 0.604 |
| CT | 4.03569 | 4.03538 | 0.008 |
| CT | 4.12777 | 4.12531 | 0.060 |

We also calculate $\mu^{\text{RMS}}$ and $\mu^{\text{LBAC}}$ metrics for these excited states and observe that their relative differences are also less than 1% and they show the same trend (signs) as $\mu^{\text{EMD}}$.

For excitations with relatively larger de-excitation effects, we choose the first triplet state of acetylene using $\omega$B97M-V as an example (which is from the Supplemental Table S5.6 in Ref. S1).

| Property name | Metric with TDA | Metric without TDA | Relative difference % |
|---|---|---|---|
| Excitation energy (eV) | 5.47 | 5.13 | 6.82 |
| $\mu^{\text{LBAC}}$ | 0 | 0 | 0 |
| $\mu^{\text{RMS}}$ | 1.92 | 1.80 | 6.67 |
| $\mu^{\text{EMD}}$ | 0.413 | 0.411 | 0.487 |

In this case, the $\mu^{\text{LBAC}}$ value keeps zero since the excitation is centrosymmetric. The change of $\mu^{\text{RMS}}$ and $\mu^{\text{EMD}}$ is in the same direction, with the fact that $\mu^{\text{RMS}}$ shows a larger deviation. This may originate from the different impacts of TDA on the real space density and transition density matrix.

Based on the two examples, we think that the influence of TDA is usually small and the main conclusions in our article will remain the same if without TDA. However, it is worth noting that the de-excitation effects might influence the real space and Hilbert space differently.

# References


(S1) Liang, J.; Feng, X.; Hait, D.; Head-Gordon, M. Revisiting the performance of time-dependent density functional theory for electronic excitations: Assessment of 43 popular and recently developed functionals from rungs one to four. *J. Chem. Theory Comput.* **2022**, *18*, 3460–3473.

(S2) Peach, M. J.; Benfield, P.; Helgaker, T.; Tozer, D. J. Excitation energies in density functional theory: An evaluation and a diagnostic test. *J. Chem. Phys.* **2008**, *128*, 044118.

(S3) Etienne, T.; Assfeld, X.; Monari, A. Toward a quantitative assessment of electronic transitions' charge-transfer character. *J. Chem. Theory Comput.* **2014**, *10*, 3896–3905.

(S4) Etienne, T.; Assfeld, X.; Monari, A. New insight into the topology of excited states through detachment/attachment density matrices-based centroids of charge. *J. Chem. Theory Comput.* **2014**, *10*, 3906–3914.

(S5) Grimme, S. Semiempirical GGA-type density functional constructed with a long-range dispersion correction. *J. Comput. Chem.* **2006**, *27*, 1787–1799.

(S6) Sun, J.; Ruzsinszky, A.; Perdew, J. P. Strongly constrained and appropriately normed semilocal density functional. *Phys. Rev. Lett.* **2015**, *115*, 036402.

(S7) Hui, K.; Chai, J.-D. SCAN-based hybrid and double-hybrid density functionals from models without fitted parameters. *J. Chem. Phys.* **2016**, *144*, 044114.

(S8) Stephens, P. J.; Devlin, F. J.; Chabalowski, C. F.; Frisch, M. J. Ab initio calculation of vibrational absorption and circular dichroism spectra using density functional force fields. *J. Phys. Chem.* **1994**, *98*, 11623–11627.

(S9) Yanai, T.; Tew, D. P.; Handy, N. C. A new hybrid exchange–correlation functional using the Coulomb-attenuating method (CAM-B3LYP). *Chem. Phys. Lett.* **2004**, *393*, 51–57.

(S10) Mardirossian, N.; Head-Gordon, M. $\omega$B97X-V: A 10-parameter, range-separated hybrid, generalized gradient approximation density functional with nonlocal correlation, designed by a survival-of-the-fittest strategy. *Phys. Chem. Chem. Phys.* **2014**, *16*, 9904–9924.

(S11) Guido, C. A.; Cortona, P.; Mennucci, B.; Adamo, C. On the metric of charge transfer molecular excitations: a simple chemical descriptor. *J. Chem. Theory Comput.* **2013**, *9*, 3118–3126.
